# Supplementary material for: Fast and Memory-Efficient Significant Pattern Mining via Permutation Testing
Source: arXiv:1502.04315 source file (2015-02-15)
Supplement: Supplementary file 1 [file appendix.tex]

\section{Bonferroni Correction and Its Improvement by Tarone}
\label{sec:app}

Among all multiple hypothesis testing procedures which control the FWER, the \emph{Bonferroni correction} is the most commonly used. It is derived, and named, after the work in \cite{Bonferroni36} but was first used in \cite{dunn1959} . It is based on a simple principle. Assume we use a rule $p_{i}\le \delta$, where $\delta$ is the \emph{corrected significance threshold}, to determine which patterns are statistically significant. Then we can write the FWER as 
% $\mathrm{FWER} = \mathrm{Pr}\left(\cup_{i=1}^{D}{\set{\left[p_{i} \le \delta\right] | H_{0}^{(i)}}}\right)$,
$\mathrm{FWER} = \mathrm{Pr}(\,\bigcup_{i=1}^{D}\mathbbm{1}[p_{i} \le \delta]\,)$,
({\bf M: please check this is correct})
where $\mathbbm{1}[\bullet]$ denotes a function which evaluates to $1$ if its argument is true and to $0$ otherwise. By applying Boole's inequality we have
% $\mathrm{FWER} \le \sum_{i=1}^{D}\mathrm{Pr}\left(\set{\left[p_{i} \le \delta\right] | H_{0}^{(i)}}\right) \le \delta D$.
$\mathrm{FWER} \le \sum_{i=1}^{D}\mathrm{Pr}(\,\mathbbm{1}[p_{i} \le \delta]\,) \le \delta D$.
Therefore, setting $\delta = \alpha/D$ controls the FWER at significance level $\alpha$. Nevertheless, this correction has an important pitfall: If the number of tests $D$ is large enough, $\delta$ might be so small that the resulting testing procedure has virtually no statistical power to detect salient patterns in the data. While that poses a challenge in general, at first it appears to be an insurmountable hurdle for statistically sound data mining. In scenarios where $D$ increases exponentially fast with the database size, $D$ might be in the order of billions or even trillions and it seems unrealistic to think that any FWER-controlling procedure could have any  statistical power remaining after correcting the significance level. Furthermore, the multiple testing problem poses a huge computational challenge as well, since carrying out a number of significance tests exponentially growing with the database size is simply not feasible.

Given a tentative corrected significance threshold $\delta$,
% and just based on the margins $x$, $n$ and $N$ of the 2x2 contingency table,
one can know that all patterns for which $\Psi(x_{i}) > \delta$ have no chance of being significant and can be pruned from the search space. We will refer to those patterns as \emph{untestable}, while those satisfying $\Psi(x_{i}) \le \delta$ will be said to be \emph{testable}. Even more importantly, because those patterns can never be significant, they do not need to be included in the Bonferroni correction factor. Precisely, let $\mathcal{I}_{T}(\delta)$ be the set of patterns testable at level $\delta$, that is, $\mathcal{I}_{T}(\delta) = \left\{i \in \left\{1,\hdots,D\right\} | \Psi(x_{i}) \le \delta \right\}$ and $m(\delta)=\left\vert \mathcal{I}_{T}(\delta) \right\vert$. Then, following the same steps used to derive the Bonferroni correction, one can prove that $\mathrm{FWER} \le \delta m(\delta)$. Thus, an improved corrected significance threshold can be found as $\delta^{*} = \max\set{\delta | \delta m(\delta) \le \alpha}$. Since $m(\delta) \ll D$ in most real-world datasets, this improvement can bring a drastic increase in statistical power.

One fundamental observation, not emphasised neither in \cite{Tarone} nor \cite{TeradaPNAS}, is that it is essential that the model under the null hypothesis for Fisher's exact test is a probability distribution conditioned on the table marginals. Otherwise, the whole method would not be mathematically sound. Since $\Psi(x_{i})$ conveys information about $x_{i}$, $n$ and $N$, if the distribution of the test statistic under the null hypothesis was not conditional on the margins, knowledge about $\Psi(x_{i})$ could potentially distort the distribution of null p-values due to ``information leaking''. Intuitively, one relies on using test statistics for which evaluating the minimum attainable p-value does not involve any magnitudes modelled as random variables under the null hypothesis or, if it does, those must be provably statistically independent of the test statistic from which the p-values are computed.

This improved Bonferroni correction, as proposed in \cite{Tarone}, would require computing $\Psi(x_{i})$ for each pattern in order to evaluate $m(\delta)$ as many times as needed in a linear search. Needless to say, in a data mining context, such approach is unfeasible except for toy examples, as it would require mining and computing the support of every single pattern in the dataset. The computational unfeasibility of the original method resulted in it being largely ignored by the data mining community until until the 2013 breakthrough paper by Terada et al.~\cite{TeradaPNAS}. There, the authors propose the Limitless-Arity Multiple-testing Procedure (LAMP), a branch-and-bound algorithm which is able to apply the method described in~\cite{Tarone} to data mining problems of the form considered in this paper.
